# Supplementary material for: Adapting Self-Supervised Representations to Multi-Domain Setups
Source: arXiv:2309.03999 source file (2023-12-13)
Supplement: Supplementary file 1 [file appendix.tex]

\appendix
\onecolumn

\setcounter{figure}{0}

\setcounter{table}{0} 

\section{Appendix}
